# Supplementary material for: Dissipative effects in odd viscous Stokes flow around a single sphere
Source: arXiv:2308.09574 ancillary file (2024-07-17)
Supplement: Supplementary file 1 [file SM_OV_final.pdf]

# Supplemental Material for "Dissipative effects in odd viscous Stokes flow around a single sphere"

Jeffrey C. Everts[1, 2, *] and Bogdan Cichocki[1]

[1] *Institute of Theoretical Physics, Faculty of Physics, University of Warsaw, Pasteura 5, 02-093 Warsaw, Poland*

[2] *Institute of Physical Chemistry, Polish Academy of Sciences, 01-224 Warsaw, Poland*

(Dated: June 10, 2024)

## CONTENTS

I. Inverse Fourier integrals 1
  I.1. General structure 1
  I.2. The case $n = 0$: real-space Green tensor 3
  I.3. The case $n = 1$: calculation of $\mathcal{L}_0 G_{\alpha\beta}(a\hat{\mathbf{r}})$ 3
  I.4. The case $n = 2$: calculation of $\mathcal{L}_1 \partial_\nu G_{\alpha\beta}(a\hat{\mathbf{r}})$ 4

II. Absence of translational-rotational and translational-dipolar coupling 5

III. Linear relations between force moments and generalised velocities 6

IV. Flow field around a translating sphere 8
  IV.1. The special case $\mathbf{U} \parallel \hat{\boldsymbol{\ell}}$ 8
  IV.2. General case 9

References 9

## I. INVERSE FOURIER INTEGRALS

In this section, we give the technical details for computing inverse Fourier integrals of the form

$$\mathcal{F}^{-1}\left[F_n\tilde{\mathbf{G}}\right](\mathbf{r}) = \int \frac{d\mathbf{k}}{(2\pi)^3}\, e^{i\mathbf{k}\cdot\mathbf{r}} F_n(ka)\tilde{\mathbf{G}}(\mathbf{k}), \quad n = 0, 1, 2. \tag{S.1}$$

We are interested in the inverse Fourier transform $\mathcal{F}^{-1}$ of the tensorial function $F_n\tilde{\mathbf{G}}$, with $\tilde{\mathbf{G}}(\mathbf{k})$ given by Eq. (4) in the main text, and $a$ is the particle radius. We consider only functions $F_n$ that do not contain poles in the entire $\mathbf{k}$ space. The integral in Eq. (S.1) is the main calculation we need to perform to obtain all results discussed in the main text. In particular, we consider functions of the forms

$$F_0(x) = 1, \quad F_1(x) = j_0(x), \quad F_2(x) = \frac{3j_1(x)}{x}.$$

It is clear the calculation for $n = 0$, Eq. (S.1) gives the real-space fundamental solution $\mathbf{G}(\mathbf{r})$, the case $n = 1$ is relevant for the problem of a translating sphere, and the case $n = 2$ is needed for the problem of a rotating sphere in linear shear flow. In this section, we compute Eq. (S.1) as much as possible without specifying $F_n$. In later sections, we will apply the result to specific cases.

### I.1. General structure

Using Eq. (4) in the main text, we realise that we can write $\bar{\mathbf{G}}(\mathbf{k})$

$$\tilde{G}_{\alpha\beta}(\mathbf{k}) = \tilde{A}_{\nu\nu}(\mathbf{k})\delta_{\alpha\beta} - \tilde{A}_{\alpha\beta}(\mathbf{k}) + \gamma\epsilon_{\alpha\beta\lambda}\tilde{A}_{\lambda\sigma}(\mathbf{k})\hat{\ell}_\sigma, \tag{S.2}$$

* jeffrey.everts@fuw.edu.pl

in terms of the tensor $\tilde{\mathbf{A}}(\mathbf{k})$ given by

$$\tilde{\mathbf{A}}(\mathbf{k}) = \frac{1}{\eta_s}\frac{\hat{\mathbf{k}}\hat{\mathbf{k}}}{k^2[1+\gamma^2(\hat{\mathbf{k}}\cdot\hat{\boldsymbol{\ell}})^2]}.$$

The inverse Fourier transform is a linear operation and, therefore, evaluating Eq. (S.1) reduces to determining $\mathcal{F}^{-1}\left[F_n\tilde{\mathbf{A}}\right](\mathbf{r})$. We adopt a cylindrical coordinate system where the $k_z$ coordinate is along the $\hat{\boldsymbol{\ell}}$ direction (i.e., $\hat{\mathbf{z}} = \hat{\boldsymbol{\ell}}$) and we also adopt cylindrical coordinates for the real-space coordinates,

$$k_x = k_\perp \cos k_\phi, \quad k_y = k_\perp \sin k_\phi, \quad k_z = k_z,$$
$$x = \rho\cos\phi, \quad y = \rho\sin\phi, \quad z = z,$$

from which we have that $\int d\mathbf{k}(...) = \int_0^{2\pi} dk_\phi \int_0^\infty dk_\perp\, k_\perp \int_{-\infty}^{\infty} dk_z(...)$ and $\mathbf{k}\cdot\mathbf{r} = k_\perp\rho\cos(k_\phi-\phi)+k_z z$. Therefore, we find

$$\mathcal{F}^{-1}\left[F_n\tilde{A}_{\alpha\beta}\right](\mathbf{r}) = \frac{1}{(2\pi)^3\eta_s}\int_0^\infty dk_\perp\, k_\perp \int_0^{2\pi} dk_\phi\, e^{ik_\perp\rho\cos(k_\phi-\phi)}\int_{-\infty}^{\infty} dk_z \frac{F_n\left(a\sqrt{k_\perp^2+k_z^2}\right)k_\alpha k_\beta e^{ik_z z}}{[k_\perp^2+(1+\gamma^2)k_z^2](k_\perp^2+k_z^2)}.$$

Clearly, in the coordinate system, the integral over $k_z$ is of the form

$$M_{m,n}(k_\perp,z) = \int_{-\infty}^{\infty} dk_z \frac{F_n\left(a\sqrt{k_\perp^2+k_z^2}\right)k_z^m e^{ik_z z}}{[k_\perp^2+(1+\gamma^2)k_z^2](k_\perp^2+k_z^2)}, \quad (k_\perp>0), \quad m=0,1,2. \tag{S.3}$$

Performing an analytical continuation in the complex plane and defining the variable $K$ where $\mathrm{Re}(K)=k_z$, we notice that we have four poles on the imaginary axis $K=\pm ik_\perp$ and $K=\pm ik_\perp\cos\psi$, where we defined the "angle" $\psi$ via $\cos\psi=(1+\gamma^2)^{-1/2}$. This is a useful definition since $\gamma>0$, which means that $0<\psi<\pi/2$. The introduction of $\psi$ will simplify things later in the calculation. Consider $z>0$. We define the contour $\mathcal{C}_R^+ = [-R,R]\cup\mathcal{K}_R^+$, with $\mathcal{K}_R^+$ a semi-arc with radius $R$ transversed counter-clockwise starting from $K_z=R$. Eq. (S.3) can be rewritten as

$$M_{m,n}(k_\perp,z) = \lim_{R\to\infty}\left(\oint_{\mathcal{C}_R^+} dK - \int_{\mathcal{K}_R^+} dK\right)\frac{F_n\left(a\sqrt{k_\perp^2+K^2}\right)K^m\cos^2\psi\, e^{iKz}}{[k_\perp^2\cos^2\psi+K^2](k_\perp^2+K^2)}, \quad (k_\perp>0,\ z>0), \quad m=0,1,2.$$

Using Jordan's lemma, we find that the integral over $\mathcal{K}_R^+$ vanishes, and we can use the residue theorem to compute Eq. (S.3). For $z<0$, we close the contour in the lower half plane. Performing calculation of the residues, we find

$$\bar{M}_{m,n}(k_\perp,z) = k_\perp^{3-m}M_{m,n}(k_\perp,z) = \frac{\pi[i\,\mathrm{sgn}(z)]^m}{\gamma^2}\left[e^{-k_\perp\cos\psi|z|}F_n(a\sin\psi)(\cos\psi)^{m-1} - e^{-k_\perp|z|}F_n(0)\right], \tag{S.4}$$

where we interpreted $F_n(0)=\lim_{x\to0}F_n(x)$ for $n=1,2$. We can use these functions to express

$$\mathcal{F}^{-1}\left[F_n\tilde{A}_{\alpha\beta}\right](\mathbf{r}) = \int_0^\infty \frac{dk_\perp}{(2\pi)^3\eta_s}\int_0^{2\pi} dk_\phi\, e^{ik_\perp\rho\cos(k_\phi-\phi)}\left[\bar{M}_{0,n}(k_\perp,z)\hat{k}_{\perp,\alpha}\hat{k}_{\perp,\beta} + 2\bar{M}_{1,n}(k_\perp,z)\hat{k}_{\perp,(\alpha}\hat{\ell}_{\beta)} + \bar{M}_{2,n}(k_\perp,z)\hat{\ell}_\alpha\hat{\ell}_\beta\right], \tag{S.5}$$

where we introduced the notation $\mathbf{k}_\perp = k_x\hat{\mathbf{x}}+k_y\hat{\mathbf{y}}$ with $\hat{\mathbf{k}}_\perp = \mathbf{k}_\perp/k_\perp$. We use the integrals,

$$\int_0^{2\pi} dk_\phi e^{ik_\perp\rho\cos(k_\phi-\phi)} = 2\pi J_0(k_\perp\rho), \quad \int_0^{2\pi} dk_\phi\, e^{ik_\perp\rho\cos(k_\phi-\phi)}\hat{\mathbf{k}}_\perp = 2\pi i J_1(k_\perp\rho)\hat{\boldsymbol{\rho}},$$
$$\int_0^{2\pi} dk_\phi\, e^{ik_\perp\rho\cos(k_\phi-\phi)}\hat{\mathbf{k}}_\perp\hat{\mathbf{k}}_\perp = 2\pi\left[\frac{J_1(k_\perp\rho)}{k_\perp\rho}(\mathbf{I}-\hat{\boldsymbol{\ell}}\hat{\boldsymbol{\ell}}) - J_2(k_\perp\rho)\hat{\boldsymbol{\rho}}\hat{\boldsymbol{\rho}}\right],$$

with $J_n$ the $n$-th order Bessel function of the first kind. In combination with Eq. (S.5) to find

$$\mathcal{F}^{-1}\left[F_n\tilde{\mathbf{A}}\right](\mathbf{r}) = \int_0^\infty \frac{dk_\perp}{(2\pi)^2\eta_s}\Bigg[\bar{M}_{0,n}(k_\perp,z)\frac{J_1(k_\perp\rho)}{k_\perp\rho}(\mathbf{I}-\hat{\boldsymbol{\ell}}\hat{\boldsymbol{\ell}}) - \bar{M}_{0,n}(k_\perp,z)J_2(k_\perp\rho)\hat{\boldsymbol{\rho}}\hat{\boldsymbol{\rho}}$$
$$+ i\bar{M}_{1,n}(k_\perp,z)J_1(k_\perp\rho)(\hat{\boldsymbol{\rho}}\hat{\boldsymbol{\ell}}+\hat{\boldsymbol{\ell}}\hat{\boldsymbol{\rho}}) + \bar{M}_{2,n}(k_\perp,z)J_0(k_\perp\rho)\hat{\boldsymbol{\ell}}\hat{\boldsymbol{\ell}}\Bigg]. \tag{S.6}$$

Eq. (S.6) together with Eqs. (S.16) and (S.2) is the most worked-result of Eq. (S.1) without specifying the form of the function $F_n$ other than that it is an analytical function.

### I.2. The case $n = 0$: real-space Green tensor

We will apply Eq. (S.6) to find the real-space fundamental solution, i.e. we set $n = 0$. Explicitly, for $A_{\alpha\beta}(\mathbf{r}) = \mathcal{F}^{-1}\left[\tilde{A}_{\alpha\beta}\right](\mathbf{r}) = \mathcal{F}^{-1}\left[F_0\tilde{A}_{\alpha\beta}\right](\mathbf{r})$. This expression can be explicitly evaluated using the integrals, where $\rho > 0$

$$\int_0^\infty dk_\perp\, e^{-bk_\perp}\frac{J_1(k_\perp\rho)}{k_\perp\rho} = \frac{\sqrt{b^2+\rho^2}-b}{\rho^2}, \quad \int_0^\infty dk_\perp\, e^{-bk_\perp}J_m(k_\perp\rho) = \frac{\rho^{-m}\left[\sqrt{b^2+\rho^2}-b\right]^m}{\sqrt{b^2+\rho^2}}, \quad \mathrm{Re}(b) > 0, \tag{S.7}$$

Furthermore, we introduce the variable $\tilde{r} = \sqrt{\rho^2 + z^2\cos^2\psi}/\cos\psi = r\sqrt{1+\gamma^2[1-(\hat{\mathbf{r}}\cdot\hat{\boldsymbol{\ell}})^2]}$, from which it follows that $\gamma^2\rho^2 = (\tilde{r}-r)(r+\tilde{r})$. Ultimately, we find

$$\mathbf{A}(\mathbf{r}) = \frac{1}{4\pi\eta_s(r+\tilde{r})}\left[\mathbf{I} - \hat{\boldsymbol{\ell}}\hat{\boldsymbol{\ell}} + \left(-1+\frac{z^2}{r\tilde{r}}\right)\hat{\boldsymbol{\rho}}\hat{\boldsymbol{\rho}} - \frac{z\rho}{r\tilde{r}}(\hat{\boldsymbol{\rho}}\hat{\boldsymbol{\ell}} + \hat{\boldsymbol{\ell}}\hat{\boldsymbol{\rho}}) + \frac{\rho^2}{r\tilde{r}}\hat{\boldsymbol{\ell}}\hat{\boldsymbol{\ell}}\right].$$

From the definition Eq. (S.2) and the fact that $\mathcal{F}^{-1}$ is a linear operator, we conclude that

$$\mathbf{G}(\mathbf{r}) = \frac{1}{4\pi\eta_s(r+\tilde{r})}\left[\frac{r}{\tilde{r}}\mathbf{I} + \left(1-\frac{z^2}{r\tilde{r}}\right)\hat{\boldsymbol{\rho}}\hat{\boldsymbol{\rho}} + \frac{z\rho}{r\tilde{r}}(\hat{\boldsymbol{\rho}}\hat{\boldsymbol{\ell}} + \hat{\boldsymbol{\ell}}\hat{\boldsymbol{\rho}}) + \left(1-\frac{\rho^2}{r\tilde{r}}\right)\hat{\boldsymbol{\ell}}\hat{\boldsymbol{\ell}} + \gamma\left(-\frac{z\rho}{r\tilde{r}}\hat{\boldsymbol{\rho}} + \frac{\rho^2}{r\tilde{r}}\hat{\boldsymbol{\ell}}\right)\cdot\boldsymbol{\epsilon}\right].$$

This form of the Green tensor is useful in some cases because, here, the cylindrical symmetry of the system is manifest. However, we can also express the above in terms of $\hat{\mathbf{r}}$ and $\hat{\boldsymbol{\ell}}$. We use the identity $r\hat{\mathbf{r}} = \rho\hat{\boldsymbol{\rho}} + z\hat{\boldsymbol{\ell}}$, from which it is straightforward to derive the dyadic identity $\rho z(\hat{\boldsymbol{\rho}}\hat{\boldsymbol{\ell}} + \hat{\boldsymbol{\ell}}\hat{\boldsymbol{\rho}}) = r^2\hat{\mathbf{r}}\hat{\mathbf{r}} - \rho^2\hat{\boldsymbol{\rho}}\hat{\boldsymbol{\rho}} - z^2\hat{\boldsymbol{\ell}}\hat{\boldsymbol{\ell}}$. Furthermore, from $\mathbf{I} = \nabla\mathbf{r}$ it follows that $\hat{\boldsymbol{\phi}}\hat{\boldsymbol{\phi}} = \mathbf{I} - \hat{\boldsymbol{\rho}}\hat{\boldsymbol{\rho}} - \hat{\boldsymbol{\ell}}\hat{\boldsymbol{\ell}}$. We thus arrive after some algebra at

$$\mathbf{G}(\mathbf{r}) = \frac{1}{4\pi\eta_s(r+\tilde{r})}\left[\mathbf{I} + \hat{\mathbf{r}}\hat{\mathbf{r}} - \left(1-\frac{r}{\tilde{r}}\right)\left(\hat{\mathbf{r}}\hat{\mathbf{r}} + \hat{\boldsymbol{\phi}}\hat{\boldsymbol{\phi}}\right) + \frac{\gamma}{\tilde{r}}\left(r\hat{\boldsymbol{\ell}} - z\hat{\mathbf{r}}\right)\cdot\boldsymbol{\epsilon}\right],$$

which is written in the main text as Eq. (5) in a coordinate-free form.

### I.3. The case $n = 1$: calculation of $\mathcal{L}_0 G_{\alpha\beta}(a\hat{\mathbf{r}})$

We proceed to compute $\mathcal{L}_0\mathbf{G}(a\hat{\mathbf{r}}) = \mathcal{F}^{-1}\left[F_1\tilde{\mathbf{G}}\right](a\hat{\mathbf{r}})$, which boils down to calculating $\mathbf{B}(a\hat{\mathbf{r}}) = \mathcal{F}^{-1}\left[F_1\tilde{\mathbf{A}}\right](a\hat{\mathbf{r}})$, such that

$$\mathcal{L}_0 G_{\alpha\beta}(a\hat{\mathbf{r}}) = B_{\nu\nu}(a\hat{\mathbf{r}})\delta_{\alpha\beta} - B_{\alpha\beta}(a\hat{\mathbf{r}}) + \gamma\epsilon_{\alpha\beta\lambda}B_{\lambda\sigma}(a\hat{\mathbf{r}})\hat{\ell}_\sigma. \tag{S.8}$$

Explicitly, it means we need to calculate

$$\begin{aligned}\mathbf{B}(a\hat{\mathbf{r}}) = \int_0^\infty \frac{dk_\perp}{(2\pi)^2\eta_s}\Bigg\{&\frac{1}{2}\bar{M}_{0,1}(k_\perp, a\cos\theta)[J_0(k_\perp a\sin\theta) + J_2(k_\perp a\sin\theta)](\mathbf{I} - \hat{\boldsymbol{\ell}}\hat{\boldsymbol{\ell}}) - \bar{M}_{0,1}(k_\perp, a\cos\theta)J_2(k_\perp a\sin\theta)\hat{\boldsymbol{\rho}}\hat{\boldsymbol{\rho}}\\ &+ i\bar{M}_{1,1}(k_\perp, a\cos\theta)J_1(k_\perp a\sin\theta)(\hat{\boldsymbol{\rho}}\hat{\boldsymbol{\ell}} + \hat{\boldsymbol{\ell}}\hat{\boldsymbol{\rho}}) + \bar{M}_{2,1}(k_\perp, a\cos\theta)J_0(k_\perp a\sin\theta)\hat{\boldsymbol{\ell}}\hat{\boldsymbol{\ell}}\Bigg\}.\end{aligned} \tag{S.9}$$

All the integrals can be computed analytically using Eq. (6.753.1) from Ref. [S1], which can easily be extended to our case that involves $|\cos\theta|$ in the exponent. For $\mathrm{Re}\,\nu > -1$, $a > 0$ and $0 < \psi < \pi/2$, we have

$$\int_0^\infty dk_\perp\, j_0(k_\perp a\sin\psi)e^{-k_\perp a|\cos\theta|\cos\psi}J_\nu(k_\perp a\sin\theta) = \begin{cases}\dfrac{1}{\nu a}\left(\tan\dfrac{\theta}{2}\right)^\nu\dfrac{\sin(\nu\psi)}{\sin\psi}, & 0 < \theta < \pi/2,\\[2ex] \dfrac{1}{\nu a}\left(\tan\dfrac{\pi-\theta}{2}\right)^\nu\dfrac{\sin(\nu\psi)}{\sin\psi}, & \pi/2 < \theta < \pi.\end{cases}$$

where we deduced the second case from the first case by using that $\sin(\pi - x) = \sin(x)$ and $\cos(\pi - x) = -\cos(x)$. The case for $\nu = 0$ follows by using that $\lim_{\nu\to 0}\sin(\nu\psi)/\nu = \psi$. Using these integrals and that $F_1(0) = 1$, we find that (S.9) reduces to

$$\mathbf{B}(a\hat{\mathbf{r}}) = \frac{1}{8\pi\eta_s a\gamma^2}\left[\left(\frac{1+\gamma^2}{\gamma}\psi - 1\right)\mathbf{I} + \left(3 - \frac{3+\gamma^2}{\gamma}\psi\right)\hat{\boldsymbol{\ell}}\hat{\boldsymbol{\ell}}\right].$$

Combining with Eq. (S.8) gives Eq. (10) of the main text.

### I.4. The case $n = 2$: calculation of $\mathcal{L}_1\partial_\nu G_{\alpha\beta}(a\hat{\mathbf{r}})$

Finally, we compute $\mathcal{L}_1\nabla\mathbf{G}(a\hat{\mathbf{r}}) = \mathcal{F}^{-1}\left[F_2\tilde{\mathbf{G}}\right](a\hat{\mathbf{r}})$, which boils down to calculating the rank 3 tensor $\mathbf{C}(a\hat{\mathbf{r}}) = \mathcal{F}^{-1}\left[F_2\nabla\tilde{\mathbf{A}}\right](a\hat{\mathbf{r}})$, such that

$$[\mathcal{L}_1\partial_\nu G_{\alpha\beta}](a\hat{\mathbf{r}}) = C_{\nu\rho\rho}(a\hat{\mathbf{r}})\delta_{\alpha\beta} - C_{\nu\alpha\beta}(a\hat{\mathbf{r}}) + \gamma\epsilon_{\alpha\beta\lambda}C_{\lambda\nu\sigma}(a\hat{\mathbf{r}})\hat{\ell}_\sigma. \tag{S.10}$$

To find an expression for $\mathbf{C}(a\hat{\mathbf{r}})$, we express

$$\mathbf{C}(\mathbf{r}) = \int_0^\infty \frac{dk_\perp}{(2\pi)^2\eta_s}\nabla\Bigg\{\frac{1}{2}\bar{M}_{0,2}(k_\perp,z)[J_0(k_\perp\rho)+J_2(k_\perp\rho)](\mathbf{I}-\hat{\boldsymbol{\ell}}\hat{\boldsymbol{\ell}}) - \bar{M}_{0,2}(k_\perp,z)J_2(k_\perp\rho)\hat{\boldsymbol{\rho}}\hat{\boldsymbol{\rho}}$$
$$+i\bar{M}_{1,2}(k_\perp,z)J_1(k_\perp\rho)(\hat{\boldsymbol{\rho}}\hat{\boldsymbol{\ell}}+\hat{\boldsymbol{\ell}}\hat{\boldsymbol{\rho}}) + \bar{M}_{2,2}(k_\perp,z)J_0(k_\perp\rho)\hat{\boldsymbol{\ell}}\hat{\boldsymbol{\ell}}\Bigg\}. \tag{S.11}$$

We need to calculate the gradient dyads before evaluating $\mathbf{r} = a\hat{\mathbf{r}}$. The most straightforward way is to use cylindrical coordinates $\nabla = \hat{\boldsymbol{\rho}}\partial_\rho + (\hat{\boldsymbol{\phi}}/\rho)\partial_\phi + \hat{\boldsymbol{\ell}}\partial_z$. In these coordinates, the only non-zero derivatives of unit vectors are $\partial_\phi\hat{\boldsymbol{\rho}} = \hat{\boldsymbol{\phi}}$ and $\partial_\phi\hat{\boldsymbol{\phi}} = -\hat{\boldsymbol{\rho}}$. Furthermore, Bessel function derivatives are $J'_\nu(z) = [J_{\nu-1}(z) - J_{\nu+1}(z)]/2$ and $J'_0(z) = -J_1(z)$, with prime denoting differentiation to the argument. Then Eq. (S.11) becomes

$$\mathbf{C}(\mathbf{r}) = \int_0^\infty \frac{dk_\perp}{(2\pi)^2\eta_s}\Bigg\{-\frac{1}{4}\bar{M}_{0,2}(k_\perp,z)k_\perp[J_1(k_\perp\rho)+J_3(k_\perp\rho)]\hat{\boldsymbol{\rho}}(\mathbf{I}-\hat{\boldsymbol{\ell}}\hat{\boldsymbol{\ell}}) - \frac{1}{2}\bar{M}_{0,2}(k_\perp,z)k_\perp[J_1(k_\perp\rho)-J_3(k_\perp\rho)]\hat{\boldsymbol{\rho}}\hat{\boldsymbol{\rho}}\hat{\boldsymbol{\rho}}$$
$$+\frac{1}{2}i\bar{M}_{1,2}(k_\perp,z)k_\perp[J_0(k_\perp\rho)-J_2(k_\perp\rho)]\hat{\boldsymbol{\rho}}(\hat{\boldsymbol{\rho}}\hat{\boldsymbol{\ell}}+\hat{\boldsymbol{\ell}}\hat{\boldsymbol{\rho}}) - \bar{M}_{2,2}(k_\perp,z)k_\perp J_1(k_\perp\rho)\hat{\boldsymbol{\rho}}\hat{\boldsymbol{\ell}}\hat{\boldsymbol{\ell}} - \frac{1}{\rho}\bar{M}_{0,2}(k_\perp,z)J_2(k_\perp\rho)\hat{\boldsymbol{\phi}}(\hat{\boldsymbol{\phi}}\hat{\boldsymbol{\rho}}+\hat{\boldsymbol{\rho}}\hat{\boldsymbol{\phi}})$$
$$+\frac{i}{\rho}\bar{M}_{1,2}(k_\perp,z)J_1(k_\perp\rho)\hat{\boldsymbol{\phi}}(\hat{\boldsymbol{\phi}}\hat{\boldsymbol{\ell}}+\hat{\boldsymbol{\ell}}\hat{\boldsymbol{\phi}}) + \frac{1}{2}\partial_z\bar{M}_{0,2}(k_\perp,z)[J_0(k_\perp\rho)+J_2(k_\perp\rho)]\hat{\boldsymbol{\ell}}(\mathbf{I}-\hat{\boldsymbol{\ell}}\hat{\boldsymbol{\ell}}) - \partial_z\bar{M}_{0,2}(k_\perp,z)J_2(k_\perp\rho)\hat{\boldsymbol{\ell}}\hat{\boldsymbol{\rho}}\hat{\boldsymbol{\rho}}$$
$$+i\partial_z\bar{M}_{1,2}(k_\perp,z)J_1(k_\perp\rho)\hat{\boldsymbol{\ell}}(\hat{\boldsymbol{\rho}}\hat{\boldsymbol{\ell}}+\hat{\boldsymbol{\ell}}\hat{\boldsymbol{\rho}}) + \partial_z\bar{M}_{2,2}(k_\perp,z)J_0(k_\perp\rho)\hat{\boldsymbol{\ell}}\hat{\boldsymbol{\ell}}\hat{\boldsymbol{\ell}}\Bigg\}.$$

To evaluate this expression for $\mathbf{r} = a\hat{\mathbf{r}}$, one has to use Eq. (6.629) from Ref. [S1] using that $j_1(x) = \sqrt{\pi/(2x)}J_{3/2}(x)$,

$$\int_0^\infty dk_\perp\, J_\mu(k_\perp a\sin\theta)e^{-k_\perp a\cos\psi|\cos\theta|}j_1(k_\perp a\sin\psi) = \begin{cases}\frac{1}{a}\sqrt{\frac{\pi}{2\sin\psi}}\Gamma(\mu+2)P_1^{-\mu}(\cos\theta)P_{\mu-\frac{1}{2}}^{-\frac{3}{2}}(\cos\psi), & z>0,\\ \frac{1}{a}\sqrt{\frac{\pi}{2\sin\psi}}\Gamma(\mu+2)P_1^{-\mu}(-\cos\theta)P_{\mu-\frac{1}{2}}^{-\frac{3}{2}}(\cos\psi), & z<0.\end{cases}$$

Here, $\Gamma$ is the gamma function, and $P_\mu^\nu$ are the associated Legendre polynomials. The case for $\pi/2 < \theta < \pi$ can be obtained by replacing $\theta \to \pi - \theta$ in the righthandside. Furthermore, we need the following integrals,

$$\int_0^\infty dk_\perp k_\perp J_\nu(k_\perp a\sin\theta)e^{-k_\perp a|\cos\theta|} = \begin{cases}\frac{|\cos\theta|}{a^2} & \nu=0,\\ \frac{\sin\theta}{a^2} & \nu=1,\end{cases}$$

$$\int_0^\infty dk_\perp k_\perp J_2(k_\perp a\sin\theta)e^{-k_\perp a|\cos\theta|} = \frac{2+|\cos\theta|}{a^2}\begin{cases}\tan^2\left(\frac{\theta}{2}\right), & z>0,\\ \tan^2\left(\frac{\pi-\theta}{2}\right), & z<0.\end{cases}$$

After determining $\mathbf{C}(a\hat{\mathbf{r}})$, we use Eq. (S.10) to find

$$32\pi\eta_s a^2\mathcal{L}_1\partial_\nu G_{\alpha\beta}(a\hat{\mathbf{r}}) = [3+3\gamma^2 f(\gamma)+6\gamma^2 g(\gamma)-5g(\gamma)]\delta_{\alpha\beta}\hat{\ell}_\nu(\hat{\boldsymbol{\ell}}\cdot\hat{\mathbf{r}}) - [7+3\gamma^2 f(\gamma)+2\gamma^2 g(\gamma)-g(\gamma)]\delta_{\alpha\beta}\xi_\nu$$
$$-\left[(5+6\gamma^2)g(\gamma)+\gamma^2 f(\gamma)-3\right]\left(\delta_{\alpha\nu}\hat{\ell}_\beta(\hat{\boldsymbol{\ell}}\cdot\hat{\mathbf{r}})+\hat{\ell}_\alpha\delta_{\beta\nu}(\hat{\boldsymbol{\ell}}\cdot\hat{\mathbf{r}})+\xi_\alpha\hat{\ell}_\beta\hat{\ell}_\nu+\xi_\beta\hat{\ell}_\alpha\hat{\ell}_\nu+\xi_\nu\hat{\ell}_\alpha\hat{\ell}_\beta\right)$$
$$+\left[(1+2\gamma^2)g(\gamma)+\gamma^2 f(\gamma)+1\right](\xi_\alpha\delta_{\beta\nu}+\delta_{\alpha\nu}\xi_\beta) - \left\{21-35g(\gamma)-3\gamma^2\left[f(\gamma)+10g(\gamma)\right]\right\}\hat{\ell}_\alpha\hat{\ell}_\beta\hat{\ell}_\nu(\hat{\boldsymbol{\ell}}\cdot\hat{\mathbf{r}})$$
$$+4\gamma\Big\{[f(\gamma)+g(\gamma)](\epsilon_{\alpha\beta\nu}(\hat{\boldsymbol{\ell}}\cdot\hat{\mathbf{r}})+\xi_\sigma\epsilon_{\alpha\beta\sigma}\hat{\ell}_\nu+\xi_\nu\epsilon_{\alpha\beta\sigma}\hat{\ell}_\sigma) - [3f(\gamma)+5g(\gamma)]\epsilon_{\alpha\beta\sigma}\hat{\ell}_\sigma\hat{\ell}_\nu(\hat{\boldsymbol{\ell}}\cdot\hat{\mathbf{r}})\Big\}. \tag{S.12}$$

Here, we used the notation $\hat{\mathbf{r}} = (\xi_x, \xi_y, \xi_z)$. In spherical coordinates $\xi_x = \cos\phi\sin\theta$, $\xi_y = \sin\phi\sin\theta$, and $\xi_z = \cos\theta$.

## II. ABSENCE OF TRANSLATIONAL-ROTATIONAL AND TRANSLATIONAL-DIPOLAR COUPLING

In the main text we have shown that the fluid velocity field of a translating sphere can be represented in terms of the singularity form Eq. (10). Here, we will show that such a form has vanishing torque and stresslet. The most convenient way to demonstrate is by first considering the response to a point force density, which defines the stress tensor of the fundamental solution $\mathbf{\Sigma}(\mathbf{r})$. Its explicit form is given by

$$\begin{aligned}\Sigma_{\alpha\beta\rho}(\mathbf{r}) = &- \delta_{\alpha\beta}\tilde{Q}_\rho(\mathbf{r}) + \eta_\mathrm{s}\left[\partial_\alpha G_{\beta\rho}(\mathbf{r}) + \partial_\beta G_{\alpha\rho}(\mathbf{r})\right] \\ &- \eta_\mathrm{o}\hat{\ell}_\sigma\left\{\epsilon_{\beta\lambda\sigma}[\partial_\lambda G_{\alpha\rho}(\mathbf{r}) + \partial_\alpha G_{\lambda\rho}(\mathbf{r})] + \epsilon_{\alpha\lambda\sigma}[\partial_\lambda G_{\beta\rho}(\mathbf{r}) + \partial_\beta G_{\lambda\rho}(\mathbf{r})] - 2\epsilon_{\lambda\mu\sigma}\partial_\lambda G_{\mu\rho}(\mathbf{r})\delta_{\alpha\beta}\right\}.\end{aligned}$$

By definition of the point-source response, we find that

$$\partial_\beta\Sigma_{\alpha\beta\rho}(\mathbf{r}) = - \partial_\alpha\tilde{Q}_\rho(\mathbf{r}) + \eta_\mathrm{s}\nabla^2 G_{\alpha\rho}(\mathbf{r}) + \eta_\mathrm{o}\epsilon_{\alpha\mu\lambda}\hat{\ell}_\sigma\partial_\sigma\partial_\mu G_{\lambda\rho}(\mathbf{r}) = -\delta_{\alpha\rho}\delta(\mathbf{r})$$

We define the vector $\mathbf{a} = \boldsymbol{\zeta}^{\mathrm{tt}}\cdot(\mathbf{U} - \mathbf{U}^\infty)$ and thus the corresponding stress tensor of the disturbance velocity field $\mathbf{v}(\mathbf{r}) = \mathbf{v}_0(\mathbf{r}) - \mathbf{U}^\infty$ in Eq. (10) is

$$\sigma_{\alpha\beta}(\mathbf{r}) = [\mathcal{L}_0\Sigma_{\alpha\beta\rho}](\mathbf{r})a_\rho.$$

We thus have the property

$$\partial_\beta\sigma_{\alpha\beta}(\mathbf{r}) = \partial_\beta[\mathcal{L}_0\Sigma_{\alpha\beta\rho}](\mathbf{r})a_\rho = \mathcal{L}_0[\partial_\beta\Sigma_{\alpha\beta\rho}](\mathbf{r})a_\rho = -\mathcal{L}_0[\delta(\mathbf{r})]a_\alpha. \tag{S.13}$$

First, we do the trivial check of computing $\mathbf{F}$. Denoting the surface of the particle by $S_\mathrm{p}$ and its interior by $V_\mathrm{p}$, we find upon using the Gauss theorem and Eq. (S.13),

$$F_\alpha = \int_{S_\mathrm{p}} dS\,\sigma_{\alpha\beta}(\mathbf{r})\xi_\beta = \int_{V_\mathrm{p}} d\mathbf{r}\,\partial_\beta\sigma_{\alpha\beta}(\mathbf{r}) = -\int_{V_\mathrm{p}} d\mathbf{r}\;\mathcal{L}_0[\delta(\mathbf{r})]a_\alpha = -a_\alpha.$$

Here $\xi_\alpha$ denotes the components of the surface normal and in the last step we used that the integral over $(\nabla^2)^n\delta(\mathbf{r})$ vanishes for $n$ a positive integer. This is indeed what we would expect since the singularity form satisfies the appropriate boundary condition. For the torque, we find

$$T_\alpha = \int_{S_\mathrm{p}} dS\,\epsilon_{\alpha\beta\lambda}x_\beta\sigma_{\lambda\nu}(\mathbf{r})\xi_\nu = \int_{V_\mathrm{p}} d\mathbf{r}\,\partial_\nu[\epsilon_{\alpha\beta\lambda}x_\beta\sigma_{\lambda\nu}(\mathbf{r})] = \int_{V_\mathrm{p}} d\mathbf{r}\,\epsilon_{\alpha\beta\lambda}x_\beta\partial_\nu\sigma_{\lambda\nu}(\mathbf{r}) = -\int_{V_\mathrm{p}} d\mathbf{r}\,\epsilon_{\alpha\beta\lambda}x_\beta\mathcal{L}_0[\delta(\mathbf{r})]a_\lambda = 0,$$

where we used that the stress tensor is symmetric in the third step and Eq. (S.13) in the fourth step. We conclude that $\boldsymbol{\zeta}^{\mathrm{tr}} = \boldsymbol{\zeta}^{\mathrm{rt}} = 0$. Finally, we compute the stresslet:

$$S_{\alpha\beta} = \frac{1}{2}\int_{S_\mathrm{p}} dS\,\{[\sigma_{\alpha\lambda}(\mathbf{r})\xi_\lambda]x_\beta + x_\alpha[\sigma_{\beta\lambda}(\mathbf{r})\xi_\lambda]\} - \frac{1}{3}\delta_{\alpha\beta}\int_{S_\mathrm{p}} dS\,[\sigma_{\rho\lambda}(\mathbf{r})\xi_\lambda]x_\rho$$

Applying Gauss' law, we find

$$S_{\alpha\beta} = \frac{1}{2}\int_{V_\mathrm{p}} d\mathbf{r}\,[x_\beta\partial_\lambda\sigma_{\alpha\lambda}(\mathbf{r}) + x_\alpha\partial_\lambda\sigma_{\beta\lambda}(\mathbf{r})] - \frac{1}{3}\delta_{\alpha\beta}\int_{V_\mathrm{p}} d\mathbf{r}\,x_\rho\partial_\lambda\sigma_{\rho\lambda}(\mathbf{r}) + \int_{V_\mathrm{p}} d\mathbf{r}\,\left[\sigma_{\alpha\beta}(\mathbf{r}) - \frac{1}{3}\delta_{\alpha\beta}\sigma_{\nu\nu}(\mathbf{r})\right] \tag{S.14}$$

First we note that

$$\begin{aligned}\int_{V_\mathrm{p}} d\mathbf{r}\,\sigma_{\alpha\beta}(\mathbf{r}) = \int_{V_\mathrm{p}} d\mathbf{r}\,\Big(&- \tilde{p}(\mathbf{r})\delta_{\alpha\beta} + \eta_\mathrm{s}[\partial_\alpha v_\beta(\mathbf{r}) + \partial_\beta v_\alpha(\mathbf{r})] \\ &-\eta_\mathrm{o}\hat{\ell}_\sigma\left\{\epsilon_{\beta\lambda\sigma}[\partial_\lambda v_\alpha(\mathbf{r}) + \partial_\alpha v_\lambda(\mathbf{r})] + \epsilon_{\alpha\lambda\sigma}[\partial_\lambda v_\beta(\mathbf{r}) + \partial_\beta v_\lambda(\mathbf{r})] - 2\epsilon_{\lambda\mu\sigma}\partial_\lambda v_\mu(\mathbf{r})\delta_{\alpha\beta}\right\}\Big) = -\delta_{\alpha\beta}\int_{V_\mathrm{p}} d\mathbf{r}\,\tilde{p}(\mathbf{r}) \\ &+ \int_{S_\mathrm{p}} dS\,\Big(\eta_\mathrm{s}[\xi_\alpha v_\beta(\mathbf{r}) + \xi_\beta v_\alpha(\mathbf{r})] - \eta_\mathrm{o}\hat{\ell}_\sigma\left\{\epsilon_{\beta\lambda\sigma}[\xi_\lambda v_\alpha(\mathbf{r}) + \xi_\alpha v_\lambda(\mathbf{r})] + \epsilon_{\alpha\lambda\sigma}[\xi_\lambda v_\beta(\mathbf{r}) + \xi_\beta v_\lambda(\mathbf{r})] - 2\epsilon_{\lambda\mu\sigma}\xi_\lambda v_\mu(\mathbf{r})\delta_{\alpha\beta}\right\}\Big)\end{aligned} \tag{S.15}$$

On the particle surface we have simple rigid-body motion, and by the spherical symmetry we thus have that

$$\int_{S_\mathrm{p}} dS\,\xi_\alpha v_\beta(\mathbf{r}) = (U_\beta - U^\infty_\beta)\int_{S_\mathrm{p}} dS\,\xi_\alpha = 0.$$

The entire second integral in Eq. (S.15) thus vanishes. Furthermore, $(1/3)\sigma_{\nu\nu}(\mathbf{r}) = -\tilde{p}(\mathbf{r})$ and together with Eq. (S.15) we conclude that the third integral in Eq. (S.14) vanishes. The final terms in Eq. (S.14) can be rewritten as before using Eq. (S.13)

$$S_{\alpha\beta} = \frac{1}{2}\int_{V_\mathrm{p}} d\mathbf{r}\,\{x_\beta\mathcal{L}_0[\delta(\mathbf{r})]a_\alpha + x_\alpha\mathcal{L}_0[\delta(\mathbf{r})]a_\beta\} - \frac{1}{3}\delta_{\alpha\beta}\int_{V_\mathrm{p}} d\mathbf{r}\,x_\rho\mathcal{L}_0[\delta(\mathbf{r})]a_\rho = 0.$$

We conclude that $\boldsymbol{\zeta}^{\mathrm{td}} = \boldsymbol{\zeta}^{\mathrm{dt}} = 0$. Vanishing of the translational-rotational and translational-dipolar components on the level of the friction problem implies that $\boldsymbol{\mu}^{\mathrm{tr}} = \boldsymbol{\mu}^{\mathrm{rt}} = 0$ and $\boldsymbol{\mu}^{\mathrm{td}} = \boldsymbol{\mu}^{\mathrm{dt}} = 0$.

## III. LINEAR RELATIONS BETWEEN FORCE MOMENTS AND GENERALISED VELOCITIES

In the main text, we defined the grand resistance matrix $\boldsymbol{\zeta}$ and the grand mobility matrix $\boldsymbol{\mu}$. In order to compute these objects, we first compute an auxiliary object, which we call the $\boldsymbol{\mathcal{M}}$ matrix, defined as

$$\begin{pmatrix}\mathbf{U}-\mathbf{U}^\infty\\ \boldsymbol{\Omega}-\boldsymbol{\Omega}^\infty\\ -\mathbf{E}^\infty\end{pmatrix} = -\begin{pmatrix}\boldsymbol{\mathcal{M}}^{\mathrm{tt}} & \boldsymbol{\mathcal{M}}^{\mathrm{tr}} & \boldsymbol{\mathcal{M}}^{\mathrm{td}}\\ \boldsymbol{\mathcal{M}}^{\mathrm{rt}} & \boldsymbol{\mathcal{M}}^{\mathrm{rr}} & \boldsymbol{\mathcal{M}}^{\mathrm{rd}}\\ \boldsymbol{\mathcal{M}}^{\mathrm{dt}} & \boldsymbol{\mathcal{M}}^{\mathrm{dr}} & \boldsymbol{\mathcal{M}}^{\mathrm{dd}}\end{pmatrix}\begin{pmatrix}\mathbf{F}\\ \mathbf{T}\\ \mathbf{S}\end{pmatrix}. \tag{S.16}$$

The $\boldsymbol{\mathcal{M}}$ matrix is valuable for performing simulations (Stokesian dynamics) when generalised to the many-body case [S2, S3]. For interpreting experiments, $\boldsymbol{\mathcal{M}}$ is less useful than $\boldsymbol{\mu}$ because typically one cannot control the value of $\mathbf{S}$ (but one can control $\mathbf{E}^\infty$). Note that $\boldsymbol{\mu}$ and $\boldsymbol{\zeta}$ follow from $\boldsymbol{\mathcal{M}}$, e.g., $\boldsymbol{\zeta} = \boldsymbol{\mathcal{M}}^{-1}$.

We established in Sec. II that there is no translational-rotational and no translational-dipolar coupling. Therefore, $\boldsymbol{\mathcal{M}}^{\mathrm{tt}} = \boldsymbol{\mu}^{\mathrm{tt}}$, $\boldsymbol{\mathcal{M}}^{\mathrm{tr}} = \boldsymbol{\mathcal{M}}^{\mathrm{rt}} = 0$ and $\boldsymbol{\mathcal{M}}^{\mathrm{td}} = \boldsymbol{\mathcal{M}}^{\mathrm{dt}} = 0$. To compute the remaning components, we will show how $[\mathcal{L}_1\nabla\mathbf{G}](a\hat{\mathbf{r}})$ is related to $\boldsymbol{\mathcal{M}}$. From Eq. (S.12), we find,

$$\begin{aligned}8\pi\eta_\mathrm{s}a^2[\mathcal{L}_1\partial_\nu G_{\alpha\beta}](a\hat{\mathbf{r}})\epsilon_{\beta\nu\lambda} &= -\gamma^2[f(\gamma)+3g(\gamma)]\epsilon_{\alpha\lambda\sigma}\hat{\ell}_\sigma(\hat{\boldsymbol{\ell}}\cdot\hat{\mathbf{r}}) - \{\gamma^2[f(\gamma)+g(\gamma)]+2\}\epsilon_{\alpha\nu\lambda}\xi_\nu\\ &\quad -\gamma[g(\gamma)-f(\gamma)]\delta_{\alpha\lambda}(\hat{\boldsymbol{\ell}}\cdot\hat{\mathbf{r}}) - \gamma[f(\gamma)+g(\gamma)](\xi_\alpha\hat{\ell}_\lambda+\xi_\lambda\hat{\ell}_\alpha) + \gamma[3f(\gamma)+5g(\gamma)]\hat{\ell}_\alpha\hat{\ell}_\lambda(\hat{\boldsymbol{\ell}}\cdot\hat{\mathbf{r}}),\end{aligned} \tag{S.17}$$

$$\begin{aligned}16\pi\eta_\mathrm{s}a^2\{\mathcal{L}_1[\partial_\nu G_{\alpha\beta}+\partial_\beta G_{\alpha\nu}]\}(a\hat{\mathbf{r}}) &= [\gamma^2 f(\gamma)+3-5g(\gamma)](\delta_{\alpha\beta}\hat{\ell}_\nu+\delta_{\alpha\nu}\delta_{\beta z})(\hat{\boldsymbol{\ell}}\cdot\hat{\mathbf{r}}) - [\gamma^2 f(\gamma)+3-g(\gamma)](\delta_{\alpha\beta}\xi_\nu+\delta_{\alpha\nu}\xi_\beta)\\ &\quad -[(5+6\gamma^2)g(\gamma)+\gamma^2 f(\gamma)-3][\hat{\ell}_\alpha\delta_{\beta\nu}(\hat{\boldsymbol{\ell}}\cdot\hat{\mathbf{r}})+\xi_\alpha\hat{\ell}_\beta\hat{\ell}_\nu+\xi_\beta\hat{\ell}_\alpha\hat{\ell}_\nu+\xi_\nu\hat{\ell}_\alpha\hat{\ell}_\beta]\\ &\quad +[(1+2\gamma^2)g(\gamma)+\gamma^2 f(\gamma)+1]\xi_\alpha\delta_{\beta\nu} - \left\{21-35g(\gamma)-3\gamma^2\left[f(\gamma)+10g(\gamma)\right]\right\}\hat{\ell}_\alpha\hat{\ell}_\beta\hat{\ell}_\nu(\hat{\boldsymbol{\ell}}\cdot\hat{\mathbf{r}})\\ &\quad +2\gamma[f(\gamma)+g(\gamma)](\xi_\lambda\hat{\ell}_\nu\epsilon_{\alpha\beta\lambda}+\epsilon_{\alpha\beta\sigma}\hat{\ell}_\sigma\xi_\nu+\xi_\lambda\hat{\ell}_\beta\epsilon_{\alpha\nu\lambda}+\epsilon_{\alpha\nu\sigma}\hat{\ell}_\sigma\xi_\beta) - 2\gamma[3f(\gamma)+5g(\gamma)](\epsilon_{\alpha\beta\sigma}\hat{\ell}_\sigma\hat{\ell}_\nu+\epsilon_{\alpha\nu\sigma}\hat{\ell}_\sigma\hat{\ell}_\beta)(\hat{\boldsymbol{\ell}}\cdot\hat{\mathbf{r}}).\end{aligned} \tag{S.18}$$

We recognise that Eqs. (S.17) and (S.18) are linear in $\hat{\mathbf{r}}$. We define the tensors $\mathbf{X}$ and $\mathbf{W}$,

$$\frac{1}{2}\mathcal{L}_1[\partial_\nu G_{\alpha\beta}(a\hat{\mathbf{r}})]\epsilon_{\beta\nu\lambda} = \xi_\sigma X_{\alpha\sigma\lambda},\qquad \frac{1}{2}\mathcal{L}_1[\partial_\nu G_{\alpha\beta}(a\hat{\mathbf{r}})+\partial_\beta G_{\alpha\nu}(a\hat{\mathbf{r}})] = \xi_\sigma W_{\alpha\sigma\beta\nu},$$

with

$$\begin{aligned}-16\pi\eta_\mathrm{s}a^2X_{\alpha\sigma\lambda} &= \gamma^2[f(\gamma)+3g(\gamma)]\epsilon_{\alpha\lambda\tau}\hat{\ell}_\tau\hat{\ell}_\sigma + \{\gamma^2[f(\gamma)+g(\gamma)]+2\}\epsilon_{\alpha\sigma\lambda} + \gamma[g(\gamma)-f(\gamma)]\delta_{\alpha\lambda}\hat{\ell}_\sigma\\ &\quad +\gamma[f(\gamma)+g(\gamma)](\delta_{\alpha\sigma}\hat{\ell}_\lambda+\hat{\ell}_\alpha\delta_{\sigma\lambda}) - \gamma[3f(\gamma)+5g(\gamma)]\hat{\ell}_\alpha\hat{\ell}_\sigma\hat{\ell}_\lambda,\\ 32\pi\eta_\mathrm{s}a^2W_{\alpha\sigma\beta\nu} &= [\gamma^2 f(\gamma)+3-5g(\gamma)](\delta_{\alpha\beta}\hat{\ell}_\nu\hat{\ell}_\sigma+\delta_{\alpha\nu}\hat{\ell}_\beta\hat{\ell}_\sigma) - [\gamma^2 f(\gamma)+3-g(\gamma)](\delta_{\alpha\beta}\delta_{\sigma\nu}+\delta_{\alpha\nu}\delta_{\sigma\beta})\\ &\quad -[(5+6\gamma^2)g(\gamma)+\gamma^2 f(\gamma)-3](\delta_{\alpha z}\delta_{\beta\nu}\hat{\ell}_\sigma+\delta_{\alpha\sigma}\hat{\ell}_\beta\hat{\ell}_\nu+\delta_{\sigma\beta}\hat{\ell}_\alpha\hat{\ell}_\nu+\delta_{\sigma\nu}\hat{\ell}_\alpha\hat{\ell}_\beta)\\ &\quad +[(1+2\gamma^2)g(\gamma)+\gamma^2 f(\gamma)+1]\delta_{\alpha\sigma}\delta_{\beta\nu} - \left\{21-35g(\gamma)-3\gamma^2\left[f(\gamma)+10g(\gamma)\right]\right\}\hat{\ell}_\alpha\hat{\ell}_\sigma\hat{\ell}_\beta\hat{\ell}_\nu\\ &\quad +2\gamma[f(\gamma)+g(\gamma)](\hat{\ell}_\nu\epsilon_{\alpha\beta\sigma}+\epsilon_{\alpha\beta\tau}\hat{\ell}_\tau\delta_{\sigma\nu}+\hat{\ell}_\beta\epsilon_{\alpha\nu\sigma}+\epsilon_{\alpha\nu\tau}\hat{\ell}_\tau\delta_{\sigma\beta}) - 2\gamma[3f(\gamma)+5g(\gamma)](\epsilon_{\alpha\beta\tau}\hat{\ell}_\tau\hat{\ell}_\nu\hat{\ell}_\sigma+\epsilon_{\alpha\nu\tau}\hat{\ell}_\tau\hat{\ell}_\beta\hat{\ell}_\sigma).\end{aligned}$$

From invoking the boundary condition on $\mathbf{v}_1^{\mathrm{D}}(\mathbf{r})$, we find

$$-\epsilon_{\alpha\sigma\rho}(\Omega_\rho-\Omega_\rho^\infty)a - E_{\alpha\sigma}^\infty a = -X_{\alpha\sigma\lambda}T_\lambda + W_{\alpha\sigma\beta\nu}S_{\nu\beta}.$$

Taking the antisymmetric and symmetric part of this equation, respectively, and contracting the antisymmetric part with $\epsilon_{\alpha\sigma\kappa}$ gives

$$\Omega_\kappa-\Omega_\kappa^\infty = \frac{1}{2a}\left(\epsilon_{\alpha\sigma\kappa}X_{[\alpha\sigma]\lambda}T_\lambda - \epsilon_{\alpha\sigma\kappa}W_{[\alpha\sigma]\beta\nu}S_{\nu\beta}\right),\quad -E_{\alpha\sigma}^\infty = \frac{1}{a}\left(-X_{(\alpha\sigma)\lambda}T_\lambda + W_{(\alpha\sigma)\beta\nu}S_{\nu\beta}\right), \tag{S.19}$$

with square brackets denoting the antisymmetric part. We provide the explicit expressions in terms of the basis tensors defined in the main text of the symmetrisation and antisymmetrisation process,

$$-16\pi\eta_s a^2\epsilon_{\alpha\sigma\kappa}X_{[\alpha\sigma]\lambda} = 2\{\gamma^2[f(\gamma)+g(\gamma)]+2\}\hat{\ell}_\lambda\hat{\ell}_\kappa + \{\gamma^2[f(\gamma)-g(\gamma)]+4\}(\delta_{\lambda\kappa}-\hat{\ell}_\lambda\hat{\ell}_\kappa) + 2\gamma f(\gamma)\epsilon_{\lambda\kappa\tau}\hat{\ell}_\tau$$
$$16\pi\eta_s a^2\epsilon_{\alpha\sigma\kappa}W_{[\alpha\sigma]\beta\nu} = -\gamma^2[f(\gamma)+3g(\gamma)]q_{\beta\nu\kappa} - 6\gamma[f(\gamma)+g(\gamma)]p^{(0)}_{\beta\nu\kappa} + 2\gamma g(\gamma)p^{(1)}_{\beta\nu\kappa},$$
$$-32\pi\eta_s a^2 X_{(\alpha\sigma)\lambda} = \gamma^2[f(\gamma)+3g(\gamma)]q_{\alpha\sigma\lambda} - 6\gamma[f(\gamma)+g(\gamma)]p^{(0)}_{\alpha\sigma\lambda} + 2\gamma g(\gamma)p^{(1)}_{\alpha\sigma\lambda},$$
$$16\pi\eta_s a^2 W_{(\alpha\sigma)\beta\nu} = 6[f(\gamma)+g(\gamma)]d^{(0)}_{\alpha\sigma\beta\nu} - [4g(\gamma)+3\gamma^2 g(\gamma)+\gamma^2 f(\gamma)]d^{(1)}_{\alpha\sigma\beta\nu} - [\gamma^2 f(\gamma)+3-g(\gamma)]d^{(2)}_{\alpha\sigma\beta\nu}$$
$$+\gamma[f(\gamma)+g(\gamma)]c^{(0)}_{\alpha\sigma\beta\nu} - \gamma[3f(\gamma)+5g(\gamma)]c^{(1)}_{\alpha\sigma\beta\nu}.$$

Comparing Eq. (S.19) with the definition of $\boldsymbol{\mathcal{M}}$, it is straightforward to express all remaining components of $\boldsymbol{\mathcal{M}}$ in terms of $\mathbf{X}$ and $\mathbf{W}$. In that way, we find the elements of the $\boldsymbol{\mathcal{M}}$ matrix. They are

$$\boldsymbol{\mathcal{M}}^{\rm rr} = \frac{1}{32\pi\eta_s a^3}\left\{[\gamma^2 n(\gamma)+4](\mathbf{I}-\hat{\boldsymbol{\ell}}\hat{\boldsymbol{\ell}}) + [2\gamma^2 m(\gamma)+4]\hat{\boldsymbol{\ell}}\hat{\boldsymbol{\ell}} - 2\gamma f(\gamma)(\boldsymbol{\epsilon}\cdot\hat{\boldsymbol{\ell}})\right\} = \frac{3}{4a^2}\boldsymbol{\mu}^{\rm tt},$$
$$\boldsymbol{\mathcal{M}}^{\rm dr} = -\frac{1}{32\pi\eta_s a^3}\left[\gamma^2 k(\gamma)\mathbf{q} - 6\gamma m(\gamma)\mathbf{p}^{(0)} + 2\gamma g(\gamma)\mathbf{p}^{(1)}\right],$$
$$\boldsymbol{\mathcal{M}}^{\rm dd} = -\frac{1}{16\pi\eta_s a^3}\left\{6m(\gamma)\mathbf{d}^{(0)} - [4g(\gamma)+\gamma^2 k(\gamma)]\mathbf{d}^{(1)} - [\gamma^2 f(\gamma)+3-g(\gamma)]\mathbf{d}^{(2)} + \gamma m(\gamma)\mathbf{c}^{(0)} - \gamma^3 h(\gamma)\mathbf{c}^{(1)}\right\},$$

with $\gamma^2 h(\gamma) = 3f(\gamma)+5g(\gamma)$. We have the symmetry relations, $\mathcal{M}^{\rm rr}_{\alpha\beta}(\hat{\boldsymbol{\ell}}) = \mathcal{M}^{\rm rr}_{\beta\alpha}(-\hat{\boldsymbol{\ell}})$, $\mathcal{M}^{\rm rd}_{\alpha\beta\nu}(\hat{\boldsymbol{\ell}}) = \mathcal{M}^{\rm dr}_{\beta\nu\alpha}(-\hat{\boldsymbol{\ell}})$, and $\mathcal{M}^{\rm dd}_{\alpha\beta\nu\sigma}(\hat{\boldsymbol{\ell}}) = \mathcal{M}^{\rm dd}_{\nu\sigma\alpha\beta}(-\hat{\boldsymbol{\ell}})$, as a result of the OCRR. The basis tensors $\mathbf{p}^{(i)}$, $\mathbf{d}^{(i)}$, $\mathbf{q}$, and $\mathbf{c}^{(i)}$ are defined in the main text. One can check that all our results for $\boldsymbol{\mathcal{M}}$ coincide to linear order in $\gamma$ with the results of Ref. [S3].

The grand mobility matrix $\boldsymbol{\mu}$ can be determined from $\boldsymbol{\mathcal{M}}$ as follows. Due to the lack of translational-rotational and translational-dipolar coupling, we identify by comparing with the $\boldsymbol{\mathcal{M}}$ matrix that $\boldsymbol{\mu}^{\rm tt} = \boldsymbol{\mathcal{M}}^{\rm tt}$, $\boldsymbol{\mu}^{\rm tr} = \boldsymbol{\mu}^{\rm rt} = 0$, and $\boldsymbol{\mu}^{\rm td} = \boldsymbol{\mu}^{\rm dt} = 0$. For the partial inversion of the rotation-dipolar "block", we write out from the definition of $\boldsymbol{\mu}$,

$$-\boldsymbol{\mu}^{\rm rr}\cdot\mathbf{T} + \boldsymbol{\mu}^{\rm rd}:\mathbf{E}^\infty = -\boldsymbol{\mathcal{M}}^{\rm rr}\cdot\mathbf{T} - \boldsymbol{\mathcal{M}}^{\rm rd}:\mathbf{S}, \quad \mathbf{S} = -\boldsymbol{\mu}^{\rm dr}\cdot\mathbf{T} + \boldsymbol{\mu}^{\rm dd}:\mathbf{E}^\infty,$$

which we can reexpress as

$$\boldsymbol{\mu}^{\rm rr} = \boldsymbol{\mathcal{M}}^{\rm rr} - \boldsymbol{\mathcal{M}}^{\rm rd}:\boldsymbol{\mu}^{\rm dr}, \quad \boldsymbol{\mu}^{\rm rd} = -\boldsymbol{\mathcal{M}}^{\rm rd}:\boldsymbol{\mu}^{\rm dd}, \quad \boldsymbol{\mathcal{M}}^{\rm dd}:\boldsymbol{\mu}^{\rm dr} = \boldsymbol{\mathcal{M}}^{\rm dr}, \quad \boldsymbol{\mathcal{M}}^{\rm dd}:\boldsymbol{\mu}^{\rm dd} = \boldsymbol{\mathcal{I}}. \tag{S.20}$$

We first calculate $\boldsymbol{\mu}^{\rm dr}$ using that $\mu^{\rm dr}_{\alpha\beta\gamma}$ is symmetric traceless in the first two indices. Therefore, we can express in terms of the tensorial basis we constructed from the main text $\boldsymbol{\mu}^{\rm dr} = \beta_1\mathbf{q} + \beta_2\mathbf{p}^{(0)} + \beta_3\mathbf{p}^{(1)}$, with to be determined coefficients $\beta_i$ $(i = 1,2,3)$. Furthermore, we introduce the shorthand notation $\boldsymbol{\mathcal{M}}^{\rm dd} = d_1\mathbf{d}^{(0)} + d_2\mathbf{d}^{(1)} + d_3\mathbf{d}^{(2)} + d_4\mathbf{c}^{(0)} + d_5\mathbf{c}^{(1)}$ and $\boldsymbol{\mathcal{M}}^{\rm dr} = c_1\mathbf{q} + c_2\mathbf{p}^{(0)} + c_3\mathbf{p}^{(1)}$. Using Eq. (S.20), and the multiplication rules

$$\mathbf{d}^{(0)}:\mathbf{q} = 0, \quad \mathbf{d}^{(0)}:\mathbf{p}^{(0)} = \mathbf{p}^{(0)}, \quad \mathbf{d}^{(0)}:\mathbf{p}^{(1)} = 0, \quad \mathbf{d}^{(1)}:\mathbf{q} = \mathbf{q}, \quad \mathbf{d}^{(1)}:\mathbf{p}^{(0)} = 0, \quad \mathbf{d}^{(1)}:\mathbf{p}^{(1)} = \mathbf{p}^{(1)},$$
$$\mathbf{d}^{(2)}:\mathbf{q} = 0, \quad \mathbf{d}^{(2)}:\mathbf{p}^{(0)} = 0, \quad \mathbf{d}^{(2)}:\mathbf{p}^{(1)} = 0, \quad \mathbf{c}^{(0)}:\mathbf{q} = -\mathbf{p}^{(1)}, \quad \mathbf{c}^{(0)}:\mathbf{p}^{(0)} = 0, \quad \mathbf{c}^{(0)}:\mathbf{p}^{(1)} = \mathbf{q},$$
$$\mathbf{c}^{(1)}:\mathbf{q} = -\mathbf{p}^{(1)}, \quad \mathbf{c}^{(1)}:\mathbf{p}^{(0)} = 0, \quad \mathbf{c}^{(1)}:\mathbf{p}^{(1)} = \mathbf{q}.$$

we find the coefficients

$$\beta_1 = \frac{c_1 d_2 - c_3(d_4+d_5)}{d_2^2 + (d_4+d_5)^2}, \quad \beta_2 = \frac{c_2}{d_1}, \quad \beta_3 = \frac{c_3 d_2 + c_1(d_4+d_5)}{d_2^2+(d_4+d_5)^2}.$$

Next, we introduce the notation

$$\boldsymbol{\mathcal{M}}^{\rm rr} = a_1\hat{\boldsymbol{\ell}}\hat{\boldsymbol{\ell}} + a_2(\mathbf{I}-\hat{\boldsymbol{\ell}}\hat{\boldsymbol{\ell}}) + a_3(\boldsymbol{\epsilon}\cdot\hat{\boldsymbol{\ell}}), \quad \boldsymbol{\mathcal{M}}^{\rm rd} = b_1\mathbf{q}^* + b_2(\mathbf{p}^{(0)})^* + b_3(\mathbf{p}^{(1)})^*,$$

where we defined the transposition of a rank 3 tensor as $[\mathbf{a}^*]_{\alpha\beta\nu} = a_{\beta\nu\alpha}$. Using the multiplication rules $\forall i,j = 0,1$,

$$(\mathbf{p}^{(0)})^*:\mathbf{p}^{(0)} = \frac{2}{3}\hat{\boldsymbol{\ell}}\hat{\boldsymbol{\ell}}, \quad \mathbf{q}^*:\mathbf{q} = (\mathbf{p}^{(1)})^*:\mathbf{p}^{(1)} = 2(\mathbf{I}-\hat{\boldsymbol{\ell}}\hat{\boldsymbol{\ell}}), \quad (\mathbf{p}^{(i)})^*:\mathbf{p}^{(j)} = 0, \quad (i\neq j),$$
$$(\mathbf{p}^{(0)})^*:\mathbf{q} = \mathbf{q}^*:\mathbf{p}^{(0)} = 0, \quad (\mathbf{p}^{(1)})^*:\mathbf{q} = -\mathbf{q}^*:\mathbf{p}^{(1)} = 2(\boldsymbol{\epsilon}\cdot\hat{\boldsymbol{\ell}}),$$

in Eq. (S.20), we find,

$$\boldsymbol{\mu}^{\rm rr} = \left(a_1 - \frac{2}{3}\beta_2 b_2\right)\hat{\boldsymbol{\ell}}\hat{\boldsymbol{\ell}} + (a_2 - 2b_1\beta_1 - 2b_3\beta_3)(\mathbf{I} - \hat{\boldsymbol{\ell}}\hat{\boldsymbol{\ell}}) + (a_3 + 2\beta_3 b_1 - 2\beta_1 b_3)(\boldsymbol{\epsilon}\cdot\hat{\boldsymbol{\ell}}).$$

For the dipolar-dipolar mobility tensor we write, $\boldsymbol{\mu}^{\rm dd} = \delta_1\mathbf{d}^{(0)} + \delta_2\mathbf{d}^{(1)} + \delta_3\mathbf{d}^{(2)} + \delta_4\mathbf{e}^{(0)} + \delta_5\mathbf{e}^{(1)}$. Using the multiplication rules

$$\mathbf{d}^{(i)} : \mathbf{d}^{(j)} = \delta_{ij}\mathbf{d}^{(i)}, \quad \mathbf{c}^{(0)} : \mathbf{c}^{(0)} = -\left(\mathbf{d}^{(1)} + 4\mathbf{d}^{(2)}\right), \quad \mathbf{c}^{(1)} : \mathbf{c}^{(1)} = -\mathbf{d}^{(1)}, \quad \mathbf{c}^{(1)} : \mathbf{c}^{(0)} = \mathbf{c}^{(0)} : \mathbf{c}^{(1)} = -\mathbf{d}^{(1)},$$

$$\mathbf{d}^{(0)} : \mathbf{c}^{(0)} = \mathbf{c}^{(0)} : \mathbf{d}^{(0)} = 0, \quad \mathbf{d}^{(1)} : \mathbf{c}^{(0)} = \mathbf{c}^{(0)} : \mathbf{d}^{(1)} = \mathbf{c}^{(1)}, \quad \mathbf{d}^{(2)} : \mathbf{c}^{(0)} = \mathbf{c}^{(0)} : \mathbf{d}^{(2)} = \mathbf{c}^{(0)} - \mathbf{c}^{(1)},$$

$$\mathbf{d}^{(0)} : \mathbf{c}^{(1)} = \mathbf{c}^{(1)} : \mathbf{d}^{(0)} = 0, \quad \mathbf{d}^{(1)} : \mathbf{c}^{(1)} = \mathbf{c}^{(1)} : \mathbf{d}^{(1)} = \mathbf{c}^{(1)}, \quad \mathbf{d}^{(2)} : \mathbf{c}^{(1)} = \mathbf{c}^{(1)} : \mathbf{d}^{(2)} = 0,$$

and Eq. (S.20), we find after some algebra,

$$\delta_1 = \frac{1}{d_1}, \quad \delta_2 = \frac{d_2}{d_2^2 + (d_4+d_5)^2}, \quad \delta_3 = \frac{d_3}{d_3^2 + 4d_4^2}, \quad \delta_4 = -\frac{d_4}{d_3^2 + 4d_4^2}, \quad \delta_5 = \frac{d_4}{d_3^2 + 4d_4^2} - \frac{d_4 + d_5}{d_2^2 + (d_4+d_5)^2}.$$

Having found a formal expressions for $\boldsymbol{\mu}$, we find the expressions listed in the main text.

## IV. FLOW FIELD AROUND A TRANSLATING SPHERE

In the case of constant translation of the sphere, we can analytically evaluate $\mathbf{v}_0(\mathbf{r})$ defined in Eq. (10) of the main text. Because we already found $\boldsymbol{\zeta}^{\rm tt}$ (see main text), we only need to evaluate $\mathcal{L}_0\mathbf{G}(\mathbf{r})$. Unlike in Sec. I.3 we do not put $\mathbf{r} = a\hat{\mathbf{r}}$ from the start and we compute

$$\mathbf{B}(\mathbf{r}) = \int_0^\infty \frac{dk_\perp}{(2\pi)^2\eta_{\rm s}}\left\{\frac{1}{2}\bar{M}_{0,1}(k_\perp,z)[J_0(k_\perp\rho) + J_2(k_\perp\rho)](\mathbf{I} - \hat{\boldsymbol{\ell}}\hat{\boldsymbol{\ell}}) - \bar{M}_{0,1}(k_\perp,z)J_2(k_\perp\rho)\hat{\boldsymbol{\rho}}\hat{\boldsymbol{\rho}}\right.$$
$$\left. + i\bar{M}_{1,1}(k_\perp,z)J_1(k_\perp\rho)(\hat{\boldsymbol{\rho}}\hat{\boldsymbol{\ell}} + \hat{\boldsymbol{\ell}}\hat{\boldsymbol{\rho}}) + \bar{M}_{2,1}(k_\perp,z)J_0(k_\perp\rho)\hat{\boldsymbol{\ell}}\hat{\boldsymbol{\ell}}\right\}, \quad \text{(S.21)}$$

from which it follows that $\mathcal{L}_0\mathbf{G}(\mathbf{r}) = \mathrm{Tr}[\mathbf{B}(\mathbf{r})]\mathbf{I} - \mathbf{B}(\mathbf{r}) + \gamma\boldsymbol{\epsilon}\cdot\mathbf{B}(\mathbf{r})\cdot\hat{\boldsymbol{\ell}}$.

### IV.1. The special case $\mathbf{U} \parallel \hat{\boldsymbol{\ell}}$

We demonstrate the calculation for $\mathbf{U} = U\hat{\boldsymbol{\ell}}$ and comment later on how to perform the calculation for general $\mathbf{U}$. In this case, we have that $\boldsymbol{\zeta}^{\rm tt}\cdot\mathbf{U} = 12\pi\eta_{\rm s}aU/[\gamma^2 m(\gamma) + 2]\hat{\boldsymbol{\ell}}$. Therefore,

$$\mathbf{v}_0(\mathbf{r}) = \frac{12\pi\eta_{\rm s}aU}{\gamma^2 m(\gamma) + 2}\left\{\mathrm{Tr}[\mathbf{B}(\mathbf{r})]\hat{\boldsymbol{\ell}} - \mathbf{B}(\mathbf{r})\cdot\hat{\boldsymbol{\ell}} + \gamma\hat{\boldsymbol{\ell}}\times[\mathbf{B}(\mathbf{r})\cdot\hat{\boldsymbol{\ell}}]\right\}. \quad \text{(S.22)}$$

All terms can be computed explicitly by using the following integrals [S1], and Eq. (S.7)

$$\int_0^\infty dk_\perp\, e^{-\alpha k_\perp} J_0(bk_\perp) j_0(ck_\perp) = \frac{1}{c}\arcsin\left(\frac{2c}{\sqrt{\alpha^2 + (b+c)^2} + \sqrt{\alpha^2 + (b-c)^2}}\right),$$

$$\int_0^\infty dk_\perp\, e^{-\alpha k_\perp} J_1(bk_\perp) j_0(ck_\perp) = \frac{c - \sqrt{c^2 - \frac{1}{4}[\sqrt{(b+c)^2 + \alpha^2} - \sqrt{(b-c)^2 + \alpha^2}]^2}}{bc},$$

for $\alpha, b, c > 0$. We introduce the dimensionless variables $\mathcal{R}_\pm$ as defined in the main text, and we find that

$$\mathrm{Tr}[\mathbf{B}(\mathbf{r})] = \frac{1}{4\pi\eta_{\rm s}\gamma a}\arcsin\left(\frac{1}{\mathcal{R}_+}\right), \quad \mathbf{B}(\mathbf{r})\cdot\hat{\boldsymbol{\ell}} = \frac{1}{4\pi\eta_{\rm s}\gamma^2}\left\{\frac{1}{\rho}\left[\mathrm{sgn}(z)\sqrt{1 - \mathcal{R}_-^2} - \frac{z}{r}\right]\hat{\boldsymbol{\rho}} + \left[\frac{1}{r} - \frac{1}{a\gamma}\arcsin\left(\frac{1}{\mathcal{R}_+}\right)\right]\hat{\boldsymbol{\ell}}\right\}.$$

Inserting in Eq. (S.22), gives Eq. (13) of the main text. Expanding $\mathbf{v}_0(\mathbf{r})$ in this case to linear order in $\gamma$ gives

$$\mathbf{v}_0(\mathbf{r}) = \left\{\left[\frac{3a}{4r}\left(1 + \frac{z^2}{r^2}\right) + \frac{a^3}{4r^3}\left(1 - \frac{3z^2}{r^2}\right)\right]\hat{\boldsymbol{\ell}} - \frac{3}{4}\frac{\rho z}{r^2}\left(\frac{a}{r} - \frac{a^3}{r^3}\right)(\gamma\hat{\boldsymbol{\phi}} - \hat{\boldsymbol{\rho}})\right\}U + \mathcal{O}(\gamma^2).$$

On the zeroth order level, we retrieve the Stokes solution, and to first order in $\gamma$ coincides with the result in Ref. [S4].

### IV.2. General case

For general $\mathbf{U}$, we need to perform the integral containing $J_2(k_\perp \rho)$ in Eq. (S.21). We need

$$\int_0^\infty dk_\perp \, e^{-\alpha k_\perp} J_2(bk_\perp) j_0(ck_\perp) = \frac{1}{4b^2 ci} \left\{ \left[ \sqrt{(\alpha - ic)^2 + b^2} - (\alpha - ic) \right]^2 - \left[ \sqrt{(\alpha + ic)^2 + b^2} - (\alpha + ic) \right]^2 \right\},$$

where we used Gradsteyn and Ryzhik Eq. (6.623.3) [S1] for complex numbers. Defining $\Delta^2 = (\alpha^2 + b^2 - c^2)/2$, we find

$$\sqrt{(\alpha \pm ic)^2 + b^2} = \pm \left( \sqrt{\sqrt{\Delta^4 + \alpha^2 c^2} + \Delta^2} \pm i\mathrm{sgn}(\alpha c) \sqrt{\sqrt{\Delta^4 + \alpha^2 c^2} - \Delta^2} \right).$$

Therefore, since $\alpha > 0$ and $c > 0$, we find

$$\int_0^\infty dk_\perp \, e^{-\alpha k_\perp} J_2(bk_\perp) j_0(ck_\perp) = -\frac{1}{b^2 c} \left( \sqrt{\sqrt{\Delta^4 + \alpha^2 c^2} + \Delta^2} - \alpha \right) \left( \sqrt{\sqrt{\Delta^4 + \alpha^2 c^2} - \Delta^2} - c \right).$$

The general full final expression for $\mathbf{v}_0(\mathbf{r})$ is lengthy and will give limited additional physical insights, so for the sake of presentation, we only quote the result to linear order in $\gamma$,

$$\mathbf{v}_0(\mathbf{r}) = \left[ \frac{3a}{4r} (\mathbf{I} + \hat{\mathbf{r}}\hat{\mathbf{r}}) + \frac{a^3}{4r^3} (\mathbf{I} - 3\hat{\mathbf{r}}\hat{\mathbf{r}}) \right] \cdot \mathbf{U} - \frac{3a}{8r} \left( 1 - \frac{a^2}{r^2} \right) \gamma \left[ \hat{\boldsymbol{\ell}} \times \mathbf{U} - 2(\hat{\mathbf{r}} \times \mathbf{U})(\hat{\mathbf{r}} \cdot \hat{\boldsymbol{\ell}}) - \hat{\mathbf{r}} \cdot (\hat{\boldsymbol{\ell}} \times \mathbf{U})\hat{\mathbf{r}} \right] + \mathcal{O}(\gamma^2),$$

which gives insights into what kind of velocity field is generated when $\mathbf{U}$ is not in the direction of $\hat{\boldsymbol{\ell}}$.


[S1] I. S. Gradshteyn and I. M. Ryzhik, *Table of integrals, series, and products* (Academic press, 2014).
[S2] J. F. Brady and G. Bossis, Annu. Rev. Fluid Mech. **20**, 111 (1988).
[S3] H. Yuan and M. Olvera de la Cruz, Phys. Rev. Fluids **8**, 054101 (2023).
[S4] T. Khain, C. Scheibner, M. Fruchart, and V. Vitelli, J. Fluid Mech. **934**, A23 (2022).
